# Supplementary material for: A Survey on Universal Design for Fitness Wearable Devices
Source: arXiv:2006.00823 source file (2020-06-01)
Supplement: Supplementary file 1 [file Appendix.tex]

\appendices
\section{Proof of the First Zonklar Equation}
RFC6356, NSDI11, the default one implemented in the kernel as well as specified in standard, i.e. LIA algorithm\cite{wischik2011design,raiciu2011improving,becke2012fairness, raiciu2009practical, raiciu2011coupled, barre2011multipath}, it is based on the NewReno algorithm(I need to check out the Reno series algorithms). Here we can also mention the predecessor of the LIA algorithm. The idea of LIA is ... Besides LIA, there are also a couple of other algorithms which, however, do not have as good performance as LIA. They are: single path TCP(Reno-SP), uncoupled multipath TCP, LIA. After this part, we could add some comparisons between them. Also it is good that I can understand the Reno related single path algorithm.\\
An evaluation of LIA: \cite{raiciu2009practical}:WRR, semi-coupled congestion control with LIA, not pareto-optimal, fair to TCP but not to other LIA flows, a comparison with coupled and uncoupled the overall outcome with many multipath flows is that the loss rates across an interconnected network
of paths will tend to equalize. This is a form of load balancing, or more generally resource pooling.  This resource pooling is even harder when RTT is different (e.g. heterogeneous network). aiming to solve resource pooling and bottle neck fairness, unfairness rate-based congestion control.\\
OLIA, CoNEXT12(proposed)\cite{khalili2013mptcp}\\ 
\cite{becke2012fairness}:uncoupled MPTCP can be unfair to single-path TCP users sharing one of the paths. fairness centric discussion. compare different approaches regarding fairness. can define testing scenarios, fairness, homo/hetero. Four algorithms:Reno-SP, Reno-MP, MPTCP within three trivial scenarios\\
BALIA\cite{peng2016multipath}\\
CoNEXT13\cite{paasch2013benefits} and our PhD paper\cite{paasch2014improving} compare those results, ICC12 also compare those features\\
\cite{singh2013enhancing}Singh et al. [182]
found that OLIA of MPTCP still has performance issues. They
presented Adapted Opportunistic Linked Increases Algorithm
(AOLIA) to ensure controlled aggressiveness of the MPTCP
subflows. In order to minimize the packet reordering delay,
they also proposed a Push-Pull-Hybrid (PSPLH) scheduler
where Pull strategy is used to allocate data segments to multiple
flows, and Push strategy is used to tune the size of the
segments dynamically.\\
\cite{khalili2013mptcp}:demonstrated that MPTCP is not Pareto-optimal because they
found that MPTCP users can be excessively aggressive toward
TCP users over congested paths even without any benefit to
the MPTCP users. They attributed the problem to the LIA
of MPTCP. To deal with the problem, they proposed an
Opportunistic Linked Increases Algorithm (OLIA) as an alternative
for LIA and proved that OLIA is Pareto-optimal and
satisfies the three design goals of MPTCP. Like LIA, OLIA
is a window-based congestion-control algorithm that couples
the increase of congestion windows and uses unmodified TCP
behavior in the case of loss. The increase part of OLIA has two
terms. The first term provides the Pareto optimality. The second
term guarantees non-flappiness6 as MPTCP with LIA and
responsiveness (i.e., the rate of algorithm convergence). OLIA
also compensates for different RTTs by adapting the window
increases as a function of RTTs.\\
\cite{le2013improving}: Improved linked increase in wireless network, rate-based\\
\cite{zhou2013goodput}:proposed CWA-MPTCP
that examines the goodput of MPTCP with bounded receive
buffers. They found that if the paths have similar end-to-end
delays, the MPTCP goodput is near optimal, otherwise the
goodput will be degraded significantly. For a wireless environment,
they proposed a Congestion Window Adaptation (CWA)
algorithm that can adjust the congestion window dynamically
for each TCP subflow so as to mitigate the variation of endto-
end path delay, maintaining similar end-to-end delays over
multiple paths. The primary idea behind CWA is that a large
delay ratio indicates that the high-delay path is overloaded.
Its congestion window needs to be decreased to relieve traffic
and reduce path delay. For wired environment with stable
end-to-end delay they proposed using a delay-aware scheduling
algorithm to predict the receiving sequence, i.e., a FPS
manner scheduler, so that packets can arrive at the receiver in
order. In fact, stable goodput with minimal variation is
preferable for QoS assurance to real-time applications.\\
\cite{li2013delayed}:packed coding; In this paper, we investigate in depth the HoL blocking
issue in MPTCP from the RTOmin point of view. We found
that the legacy setting of RTOmin is the main cause of the
MPTCP performance degradation in the presence of timeouts.
In order to eliminate the performance degradation of MPTCP,
we propose a novel, effective, and safe Delayed ACK scheme.
The new Delayed ACK allows removing the constraint of
RTOmin at the sender while reserving the Delayed ACK
function at the receiver. It incurs little processing overhead and
no extra traffic overhead at all. Through a wide-area evaluation
using simulation, e.g, in data center, local area and Internet
wide network environments, we show that our solution could
effectively reduce the required aggregate buffer. For example,
the use of the new Delayed ACK in MPTCP could reduce
the required aggregate buffer with one- or even two-order of
magnitude in high speed networks.\\
\cite{yang2013non}:regenation barely happens. Solve the blocking\\
\cite{paasch2012exploring}: enable unchanged applications to benefit from offloading. Explore three different types of modes. High throughput but at high energy cost, decrease the latency, smooth handover\\

\section{}
\cite{iyengar2006concurrent}: a thorough study\\
\cite{dreibholz2010applying}:it considers resource pooling, the legacy sctp does not, Standard SCTP – as defined by its RFC [1] – transmits user data via a selected primary path. The idea of CMT for SCTP is to utilize all available paths. gives a new definition of rp. the intergral congestion control not only for fairness, but also be proactive for congestion\\
\cite{shailendra2011improving}: also work on the resource pooling via congestion control\\
\cite{dreibholz2011impact}: version 2 of the previous ones, considering different path characteristics\\
\cite{becke2013comparison}: MPTCP is better in a way that it uses the mesh path in management, while sctp used one path per interface\\
\cite{shailendra2013implementation}: math matical optimization in sctp min max optimization\\
\cite{cao2014tcp}: TCP friendly, wireless network, weightted congestion window\\
\textbf{Do not forget to mention control plane and data plane.}
\subsubsection{\textbf{Control plane}}
Creating and destroying the subflows and other connection level information\\
From an implementation viewpoint, MultiPath TCP raises several important
challenges. We have analyzed several of them based on our experience in implementing
the first MultiPath TCP implementation in the Linux kernel. In
particular, we have shown how such an implementation can be structured and
discussed how buffer management must be adapted due to the utilization of
multiple subflows. We have analyzed the performance of our implementation in
the HEN testbed and shown that the coupled congestion control scheme is more
fair than the standard TCP congestion control scheme. We have also evaluated
the impact of the delay on the receive buffers and the throughput and showed\cite{bonaventure2016multipath}. \\
Standard\cite{ford2013tcp}\\
\cite{ford2011architectural}: Standard\\
\cite{raiciu2012hard}:not about congestion control but about the protocol itself. The architecture: congestion control, flow control, implementation. Opportunistic retransmission and penalitied subflow, talk about receive buffer\\
have two figures of connection initiated and connection terminated. signaling
\textbf{Use case: experimental verification}\\
\cite{mehani2015early}: an early look of MPTCP deployment host;\\
\cite{diop2012qos}: quality of service oriented MPTCP;\\
\cite{kuhn2014daps}: alleviate buffer blocking;\\
\cite{wallace2014concurrent}: modeling the congestion control environment with markrov chain;\\
\cite{paasch2013benefits}:This paper has demonstrated the benefits of applying experimental
design to evaluate and improve the reference implementation of
an IETF protocol. Applying it to real implementations enables us
to understand the impact of implementation heuristics such as autotuning
that are often neglegcted in simulation models.\\
\cite{raiciu2010data,raiciu2011improving}:Linked increase, the use in data center\\
\cite{han2016should}: should we surf the mobile web using MPTCP all the time?
